# Supplementary material for: Automated Repair of Unrealisable LTL Specifications Guided by Model Counting
Source: arXiv:2105.12595 source file (2023-04-14)
Supplement: Supplementary file 1 [file appendix.tex]

% \begin{appendix}
% \renewcommand{\thesection}{\Alph{section}}%
% \section{Threats to Validity}

% \end{appendix}
\appendix
\section{Threats to Validity}
% \label{sec:theats-to-validity}
Threats to internal validity concern the implementation of our approach, which includes third-party libraries. We mitigate this risk through several repetitions of various experiments and manual checking of the results. To compare with related approaches, we reuse their existing implementations. To validate our approximate model counting method, we re-implemented an established exact model counter, which we validated by manually checking the results for several examples. 
To mitigate external validity threats, we selected independent case studies from various sources (the literature and two unrelated synthesis benchmarks). Only additional experimentation can further alleviate this threat, facilitated by our open-source implementation. Nevertheless, we are confident that our key conclusions remain, i.e., 1) our approach can produce more solutions than random baselines, and 2) it generates many unique solutions compared to alternative methods while supporting a larger fragment of LTL.
In practice, any generated repair needs to be validated by a domain expert wrt. How reasonable the assumptions are and the compatibility of the guarantees with the system requirements. Also, we should have studied the readability of the generated repairs and how easily engineers could understand the flaw in the unrealisable specification. Explainability is an exciting direction that we hope to follow in future work.
Benchmark \changing{SYNTECH15}~\cite{Maoz+2019,SpectraRepo} provides 15 unrealisable specifications in GR(1). Only the cases Humanoid458, GyroV1, and GyroV2 do not use past time operators. Thus, to analyse all the cases in the data set, we translate the remaining 12 cases to pure future-time LTL specifications. We did it manually since automated translation from Past-LTL to LTL may produce an exponential formula unsuitable for analysis~\cite{Gabbay1987}. Since manual translation is error-prone, we mitigate this threat by verifying with NuSMV that the translated specifications are equivalent to the original unrealisable specifications. 
After checking for realisability with Strix, we realised 7 of the translated specifications were realisable.  
The work of~\cite{Maoz+2019}, where \changing{SYNTECH15} was introduced, uses Spectra~\cite{SpectraRepo} as a synthesis tool, while in our case, we use Strix~\cite{Meyer+2018}. We analyse with NuSMV the equivalence between the semantics given by Spectra and Strix to the reactive specifications, and we find that they are not precisely equivalent. That explains why some equivalent translated specifications are realisable in Strix but unrealisable in Spectra. 
The translated specifications are publicly available in the replication package provided to mitigate these threats
